# Supplementary material for: Optimal Source-Based Filtering of Malicious Traffic
Source: arXiv:1006.1165 source file (2010-06-07)
Supplement: Supplementary file 1 [file appendix.tex]

\section*{Appendix A: Proof of Theorem \ref{theorem}}

%\begin{theorem} The optimization problem FLOODING, in Eq.(\ref{P3-OF})-(\ref{P3-coverage}), is %NP-Hard.\end{theorem}

\begin{proof}
It is obvious that FLOODING is in $\mathcal{NP}$. 

To prove that it is also $\mathcal{NP}$-hard, we consider the KP problem with a cardinality constraint:
%\begin{align}\label{1.5KP-OF} %\hspace{2.5cm}
%\max \sum_{ip \in I} p_{ip} x_{ip}&&\\
%\label{1.5KP-capacity} \text{s.t.} \sum_{ip \in I} w_{ip} x_{ip}  \leq C_1&&\\
%\label{1.5KP-cardinality}    \sum_{ip \in I}  x_{ip}  = k &&
%%\label{1.5KP-domain}      x_{ip}  \in \{0,1\} 	\quad && \forall ip \in \{1,\dots,N\}
%\end{align}
\begin{align}\label{1.5KP-OF} %\hspace{2.5cm}
\max \sum_{ip \in I} p_{ip} x_{ip}, \quad \text{s.t.} \sum_{ip \in I} w_{ip} x_{ip}  \leq C_1 \text{~and~}
\sum_{ip \in I}  x_{ip}  = k 
%\label{1.5KP-domain}      x_{ip}  \in \{0,1\} 	\quad && \forall ip \in \{1,\dots,N\}
\end{align}
which is known to be $\mathcal{NP}$-hard \cite{KPbook}, and we show that it reduces to FLOODING.
First, mote that any solution of the above
problem that uses $F< F_{max}$ filters can be transformed to another feasible solution with
exactly $F_{max}$ filters.\footnote{This can be proved by referring to the LCP-tree structure. Given a solution, $S$, with $F<F_{max}$ filters, (until $F\leq N$) there exist always a filter can be replaced by two filters, corresponding to the leaves in the tree.
The solution constructed in such a way, has $F+1$ filters, keep on blocking all IPs that were blocked in $S$, and has value which is less or equal to the value of $S$.}
Therefore, the inequality in constraint (\ref{P3-cardinality}) can be replaced by an equality without
affecting the value of the optimal solution. Second, we define $\bar x_{p/l}= 1- x_{p/l} $, $\bar F_{max} =\Big(\sum_{p/l}1\Big) - F_{max}$ and we rewrite the above problem:
%\begin{align}\label{P3b-OF}
%\hspace{2.5cm}\max \sum_{l \leq r} g_{p/l} \bar x_{p/l}&&
%\end{align}
%\vspace{-0.3cm}
%s.t.
%\vspace{-0.3cm}
%\begin{align}
%\label{P3b-cardinality} \sum_{p/l} \bar x_{p/l} & = \bar F_{max}&&\\
%\label{P3b-capacity}    \sum_{p/l}\Big( g_{p/l} + b_{p/l}\Big) \bar x_{p/l} &\leq C && \\
%\label{P3b-coverage}   \sum_{p/l : i\in p/l} x_{p/l} & \leq 1\quad&&\forall i\in \mathcal{BL} && 
%\label{P3b-domain}      x_{p/l} & \in \{0,1\} 	\quad && \forall p/l
%\end{align}
\begin{align}\label{P3b-OF}
&\max \sum_{l \leq r} g_{p/l} \bar x_{p/l} ~ \text{s.t. :}\sum_{p/l} \bar x_{p/l} = \bar F_{max}, \\
\label{P3b-constraints}
&\sum_{p/l}\Big( g_{p/l} + b_{p/l}\Big) \bar x_{p/l} \leq C, ~\sum_{p/l : i\in p/l} \bar x_{p/l} \leq 1~\forall i\in \mathcal{BL}
\end{align}
\vspace{-0.1cm}
For a given instance of Problem (\ref{1.5KP-OF}), we construct an equivalent instance of Problem
 (\ref{P3b-OF})-(\ref{P3b-constraints}) by introducing the following mapping. For $i=1,\dots,N$: $- \bar g_{ii} = p_{ip}$, $ (g_{ii} + b _{ii})=w_{ip}$. For
 $p/l$ that is not in the blacklist:  $\bar g_{p/l} = 0$ and $(g_{p/l} + b _{p/l}) = C + 1$. Moreover, we assign $\bar F_{max} = k$ and $C = C_1$.
With this assignment a solution to the KP problem (\ref{1.5KP-OF}) can be obtained by solving FLOODING and then taking the values of variables $x_{p/l}$ s.t $p/l$ is in the blacklist. %\hfill $\blacksquare$
\end{proof}
